# Supplementary material for: Comparing Importance Sampling Based Methods for Mitigating the Effect of Class Imbalance
Source: arXiv:2402.18742 source file (2024-02-28)
Supplement: Supplementary file 1 [file 1_suppl.tex]

\clearpage
\setcounter{page}{1}
\maketitlesupplementary

\section*{Appendix}
\label{sec:appendix}
% In this appendix, we include the full results of experiments on ADE20K and Planet.

% \begin{figure}[h!]
%     \centering
%     \includegraphics[scale=0.75]{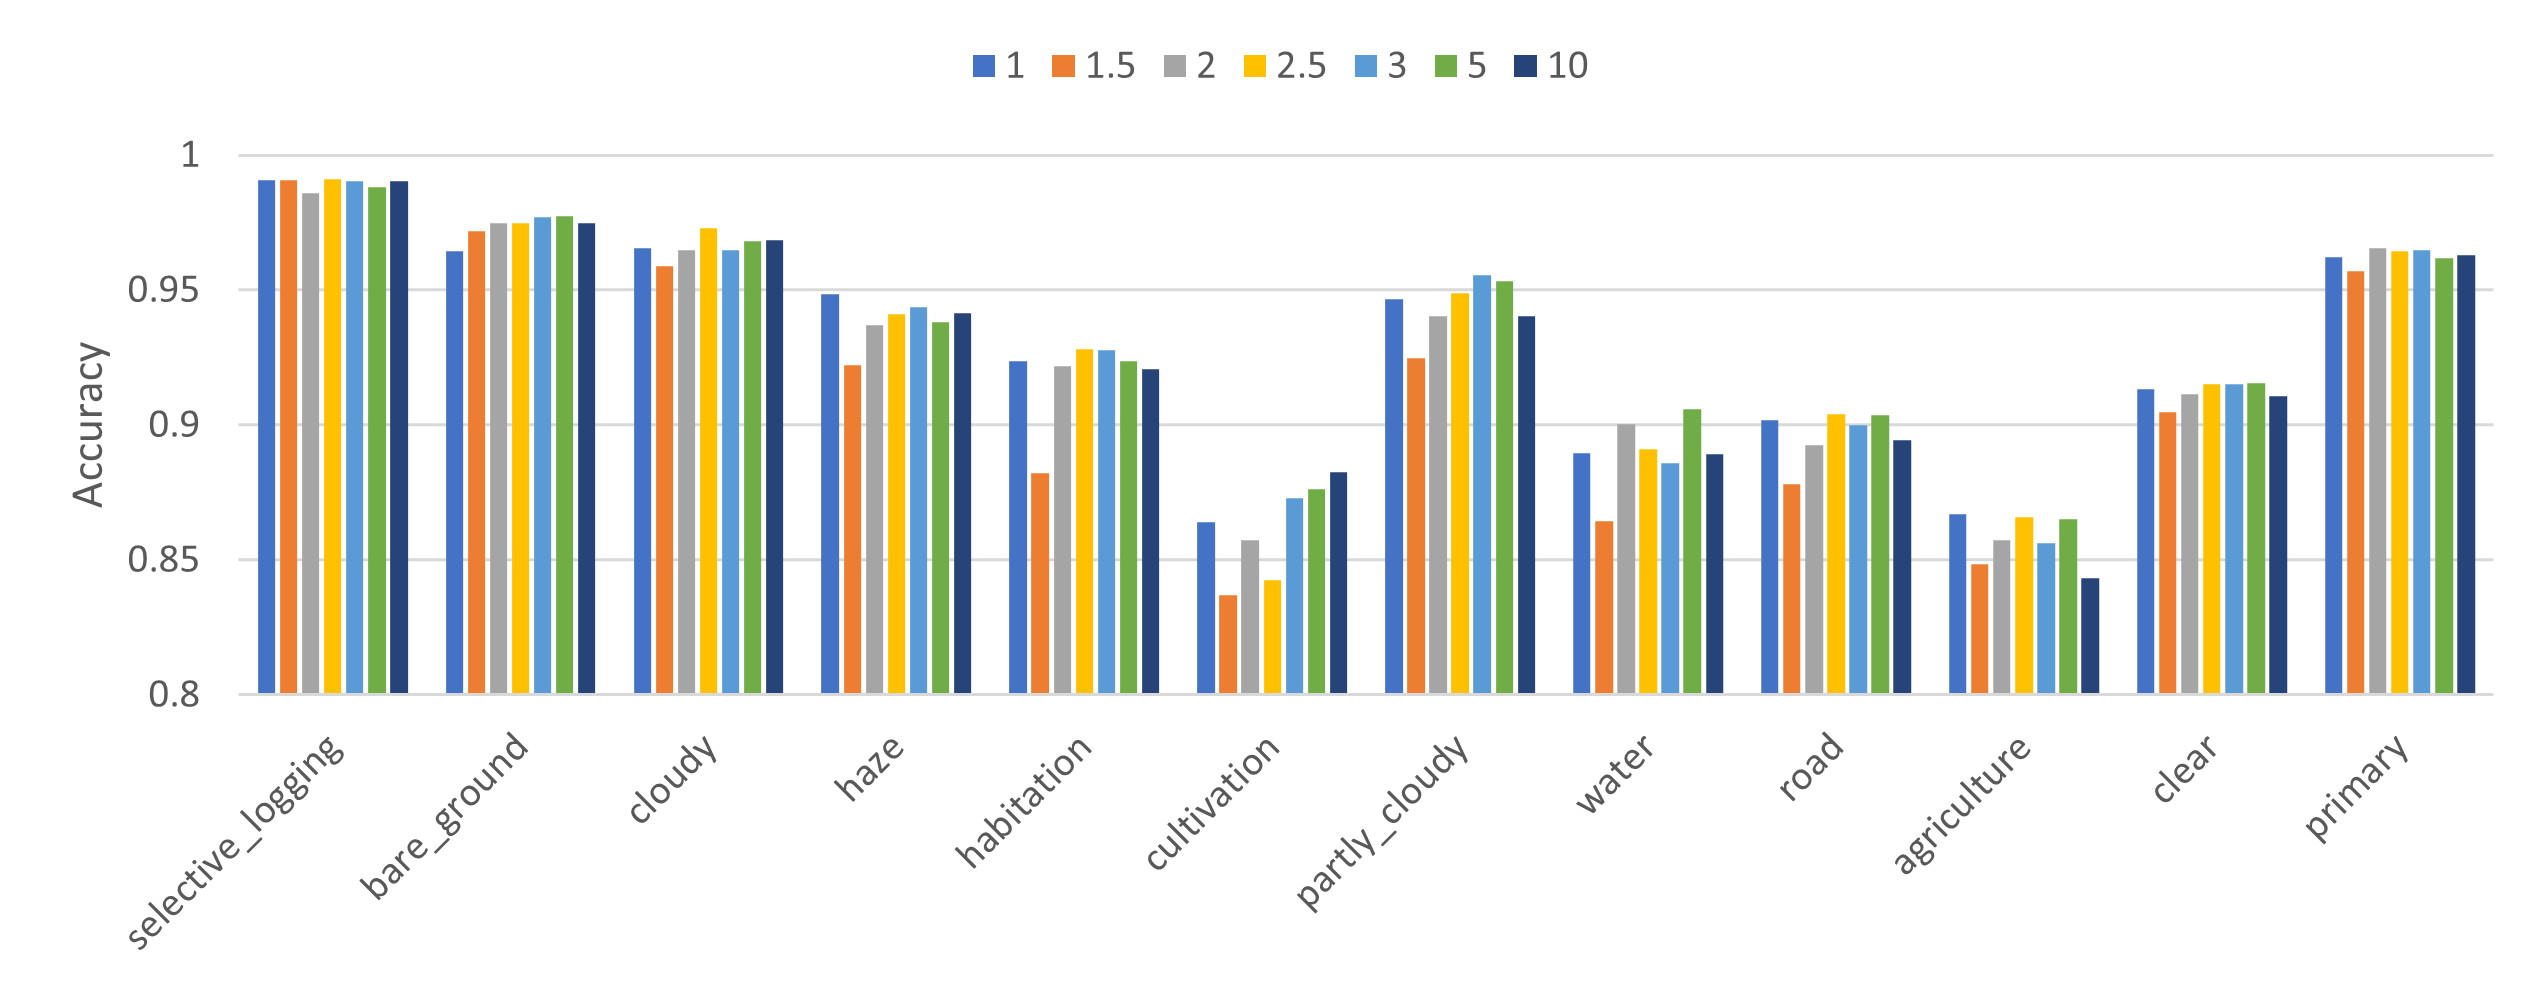}
%     \caption{\textbf{Up-weighting accuracy on the remaining classes in Planet when using CLIP.}}
%     \label{fig:clip_for_loss_nr}
% \end{figure}

% \begin{figure}[h!]
%     \centering
%     \includegraphics[scale=0.75]{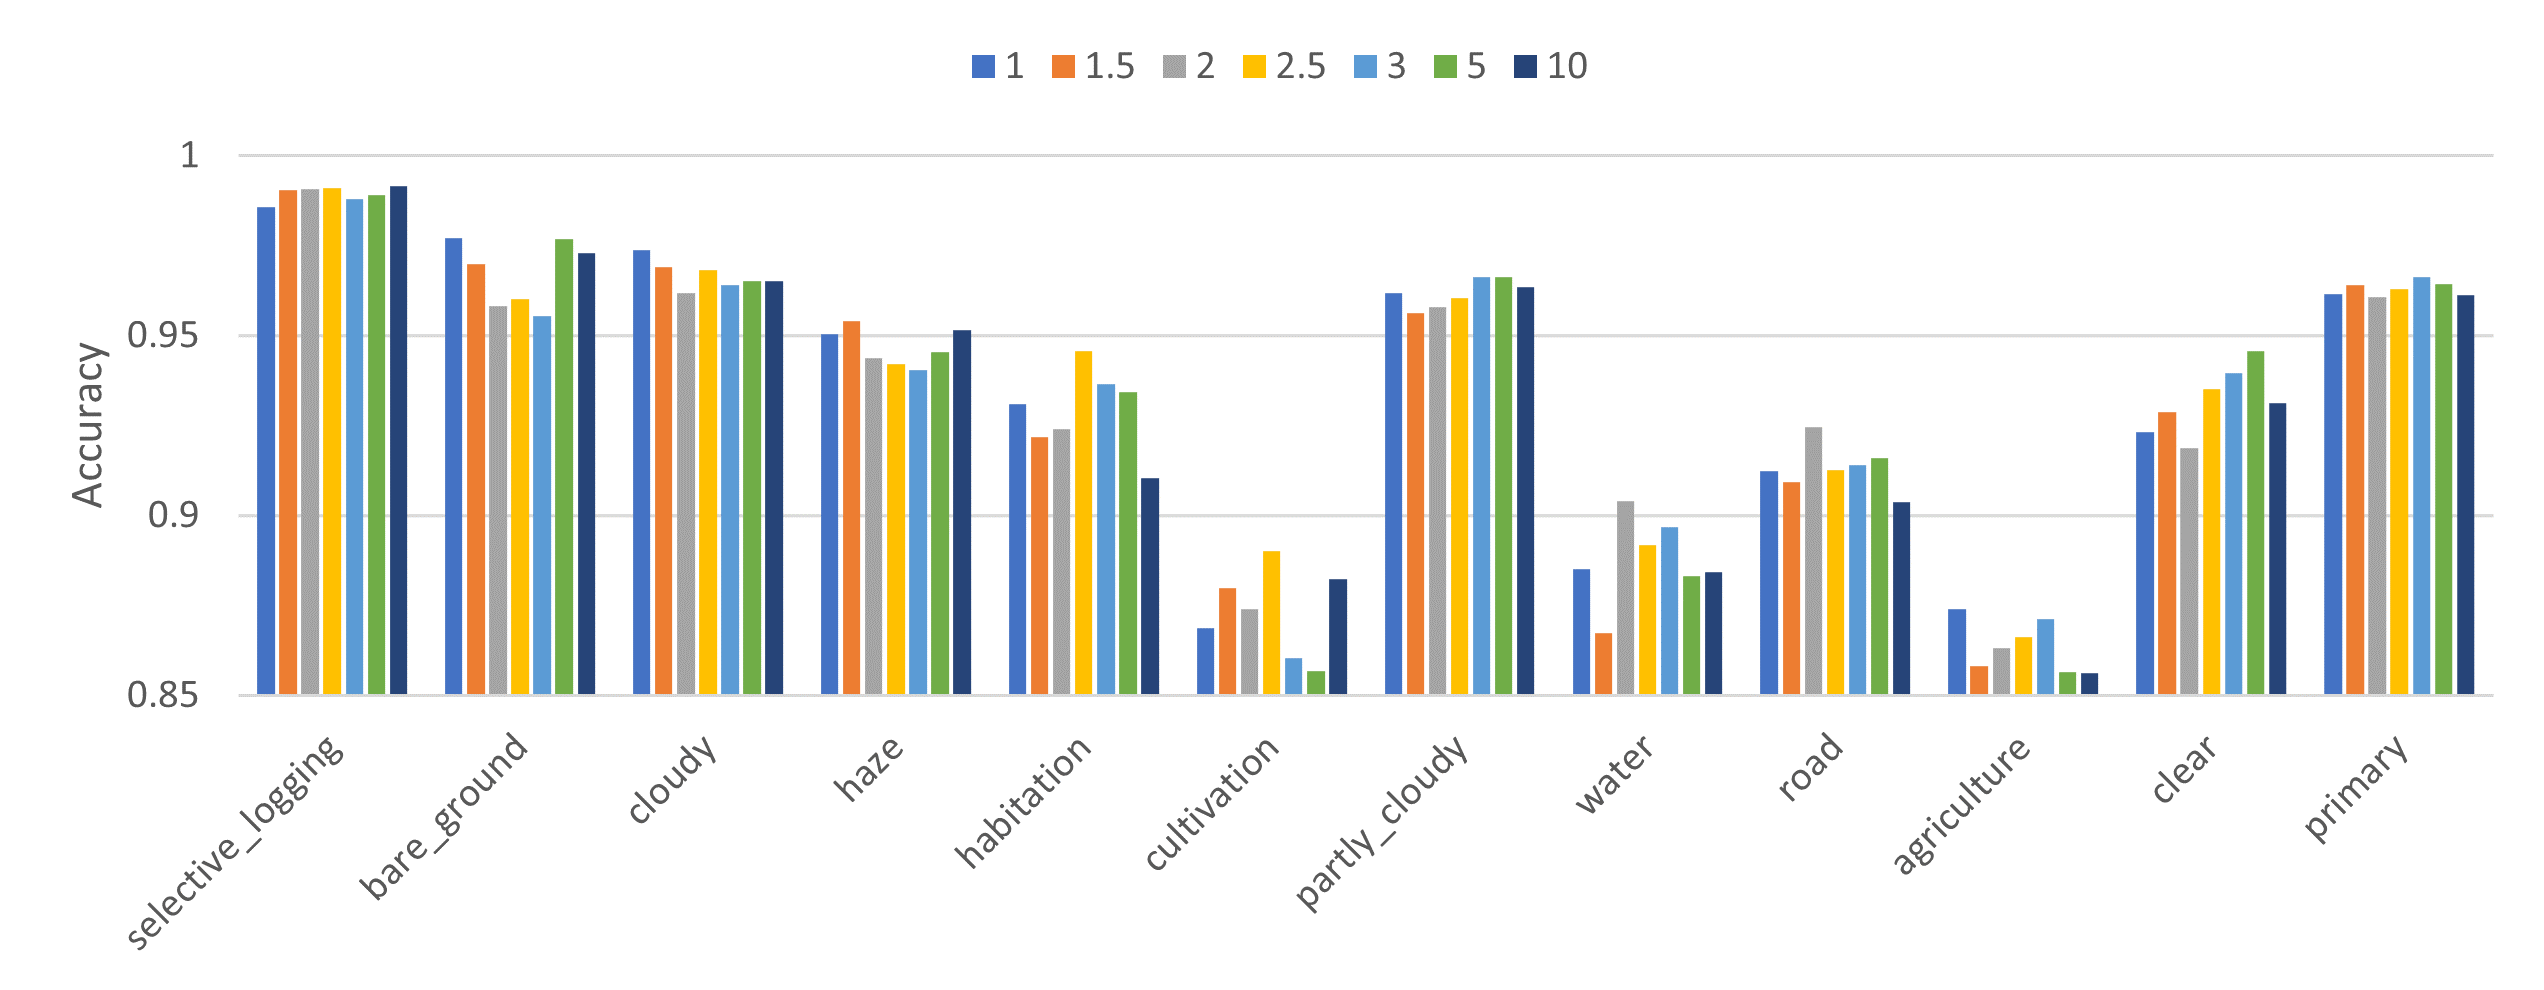}
%     \caption{\textbf{Up-weighting accuracy on the remaining classes in Planet when using ResNet-18.}}
%     \label{fig:resnet_for_loss_nr}
% \end{figure}

% \begin{figure}[h!]
%     \centering
%     \includegraphics[scale=0.75]{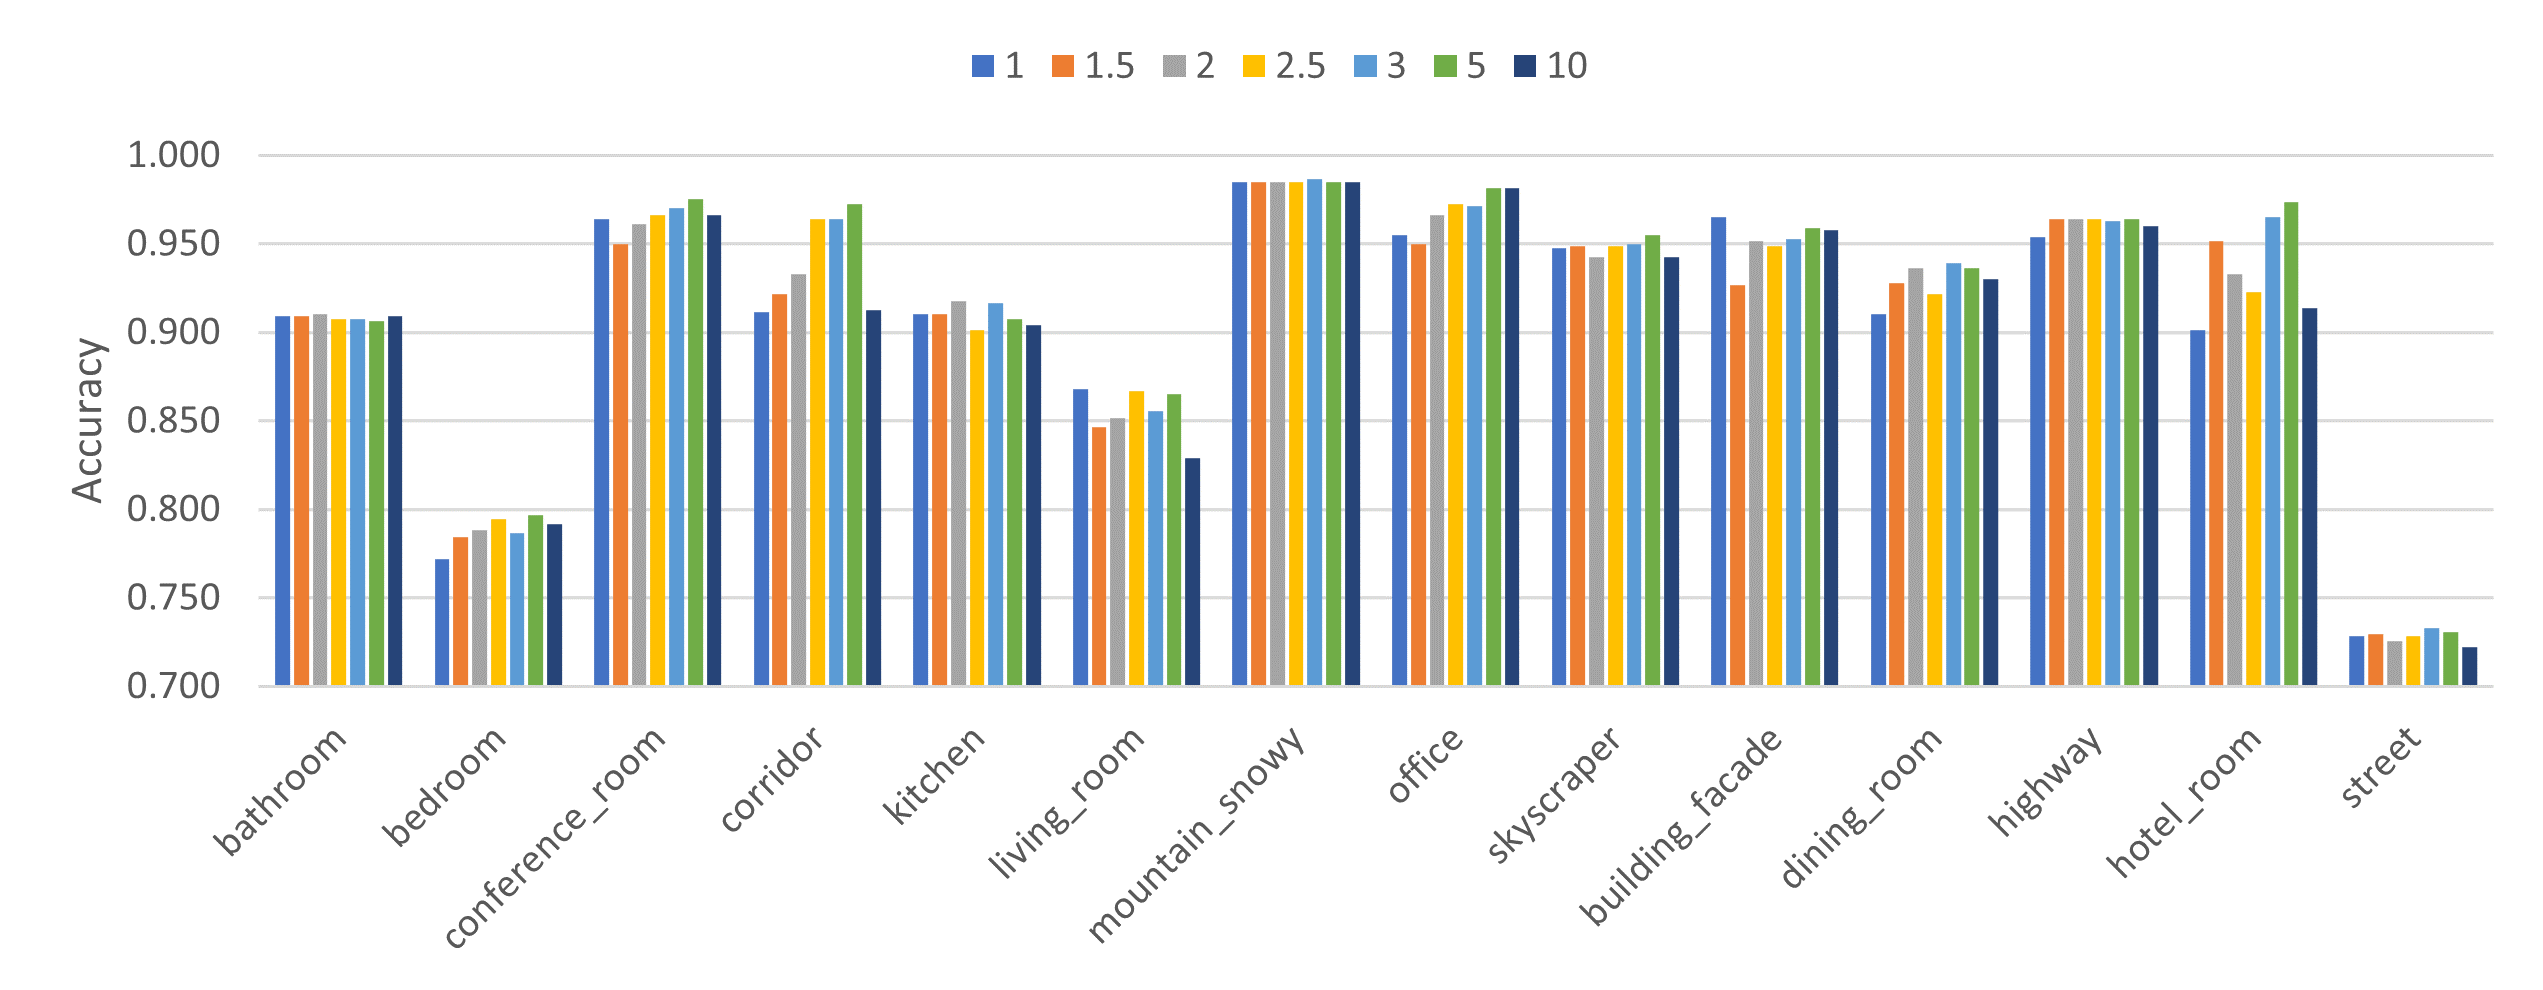}
%     \caption{\textbf{Up-weighting accuracy on the remaining classes in ADE20K when using CLIP.}}
%     \label{fig:clip_ade_loss_nr}
% \end{figure}
\textbf{1. Loss up-weighting results} \\

These are the loss up-weighting results on ADE20K for the remaining classes.

\begin{figure}[h!]
    \centering
    \includegraphics[scale=0.4]{figures/clip_ade_loss_nr.png}
    \caption{\textbf{Up-weighting accuracy on the remaining classes in ADE20K when using CLIP.}}
    \label{fig:clip_ade_loss_nr}
\end{figure}

% \begin{figure}[h!]
% \centering
%     \begin{subfigure}{0.9\linewidth}
%          \centering
%          \includegraphics[width=\linewidth]{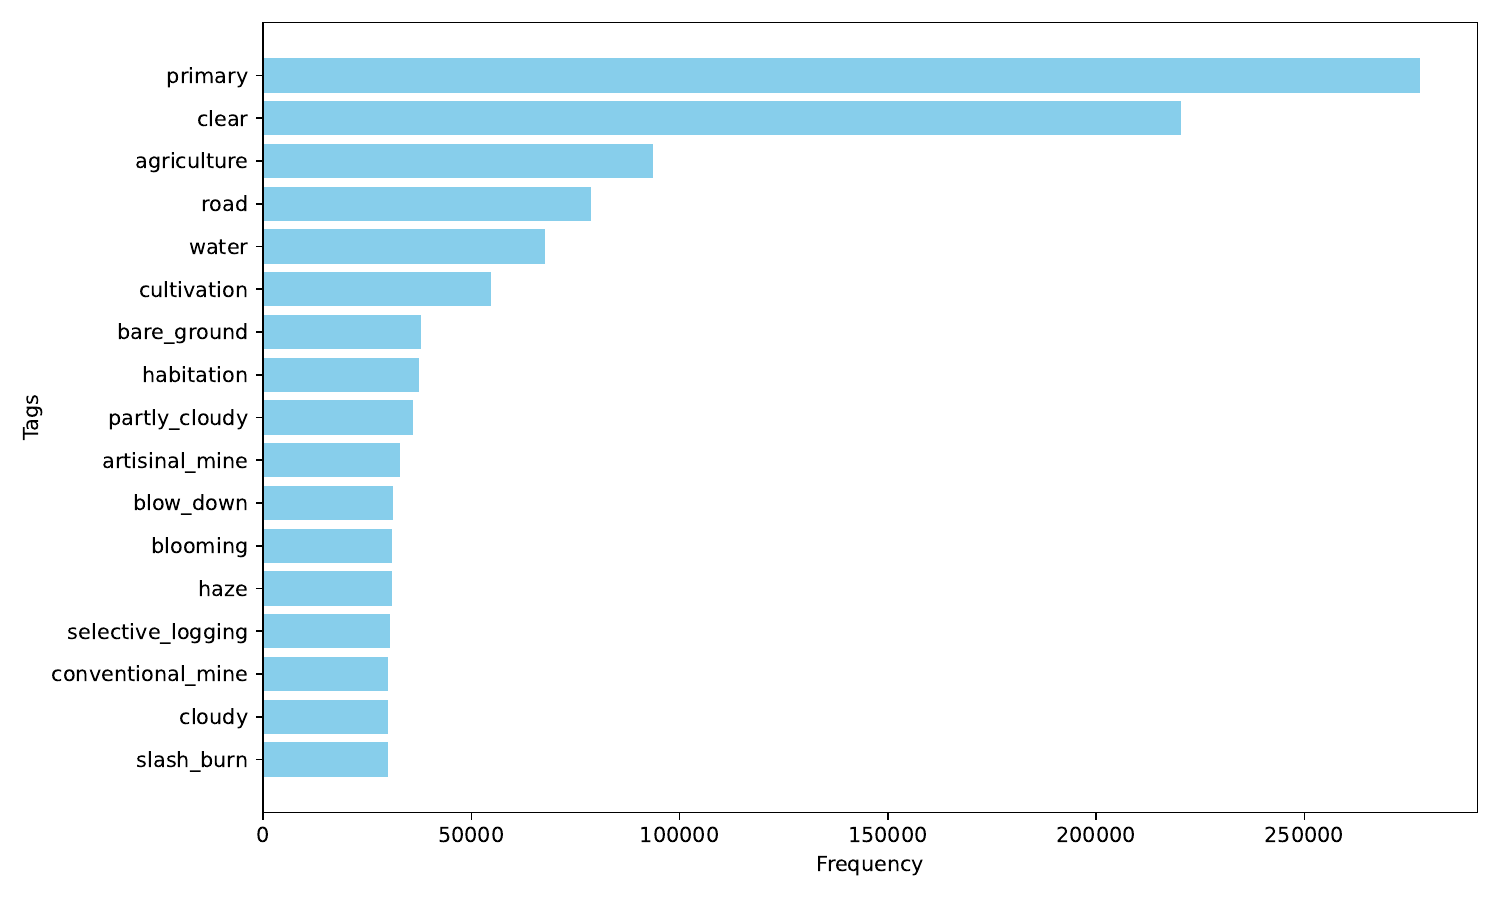}
%          \caption{\textbf{Oversampling on Planet.}}
%          \label{fig:for_oversamp_dist}
%     \end{subfigure}

%     \begin{subfigure}{0.9\linewidth}
%          \centering
%          \includegraphics[width=\linewidth]{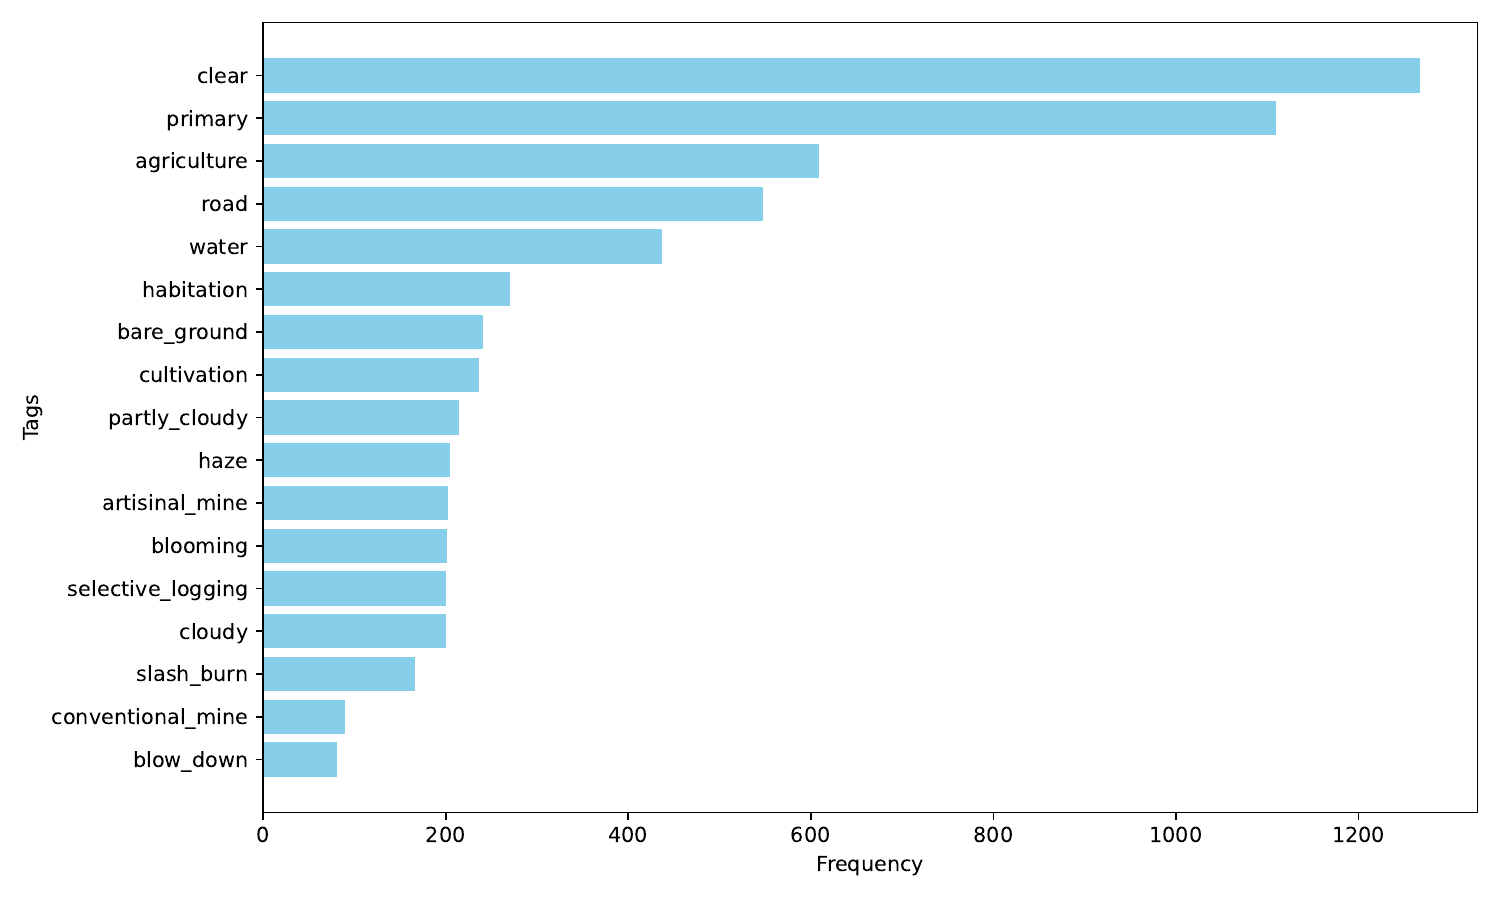}
%          \caption{\textbf{Undersampling on Planet.}}
%          \label{fig:for_undersamp_dist}
%     \end{subfigure}
%     \caption{\textbf{Sampling}}
%     \label{fig:for_sample}
% \end{figure}

% \vspace{2em}
\textbf{2. Additional Experimentation} \\

Previously, we tested a variant of undersampling and oversampling on ADE20K which is not described in the main paper.
These results are not related to the methods or results presented in the main paper. Further, the results do not show a clear trend and do not contribute substantially towards our understanding; they are included for completeness.

\begin{figure}[h!]
\centering
    \begin{subfigure}{0.6\linewidth}
         \centering
         \includegraphics[width=\linewidth]{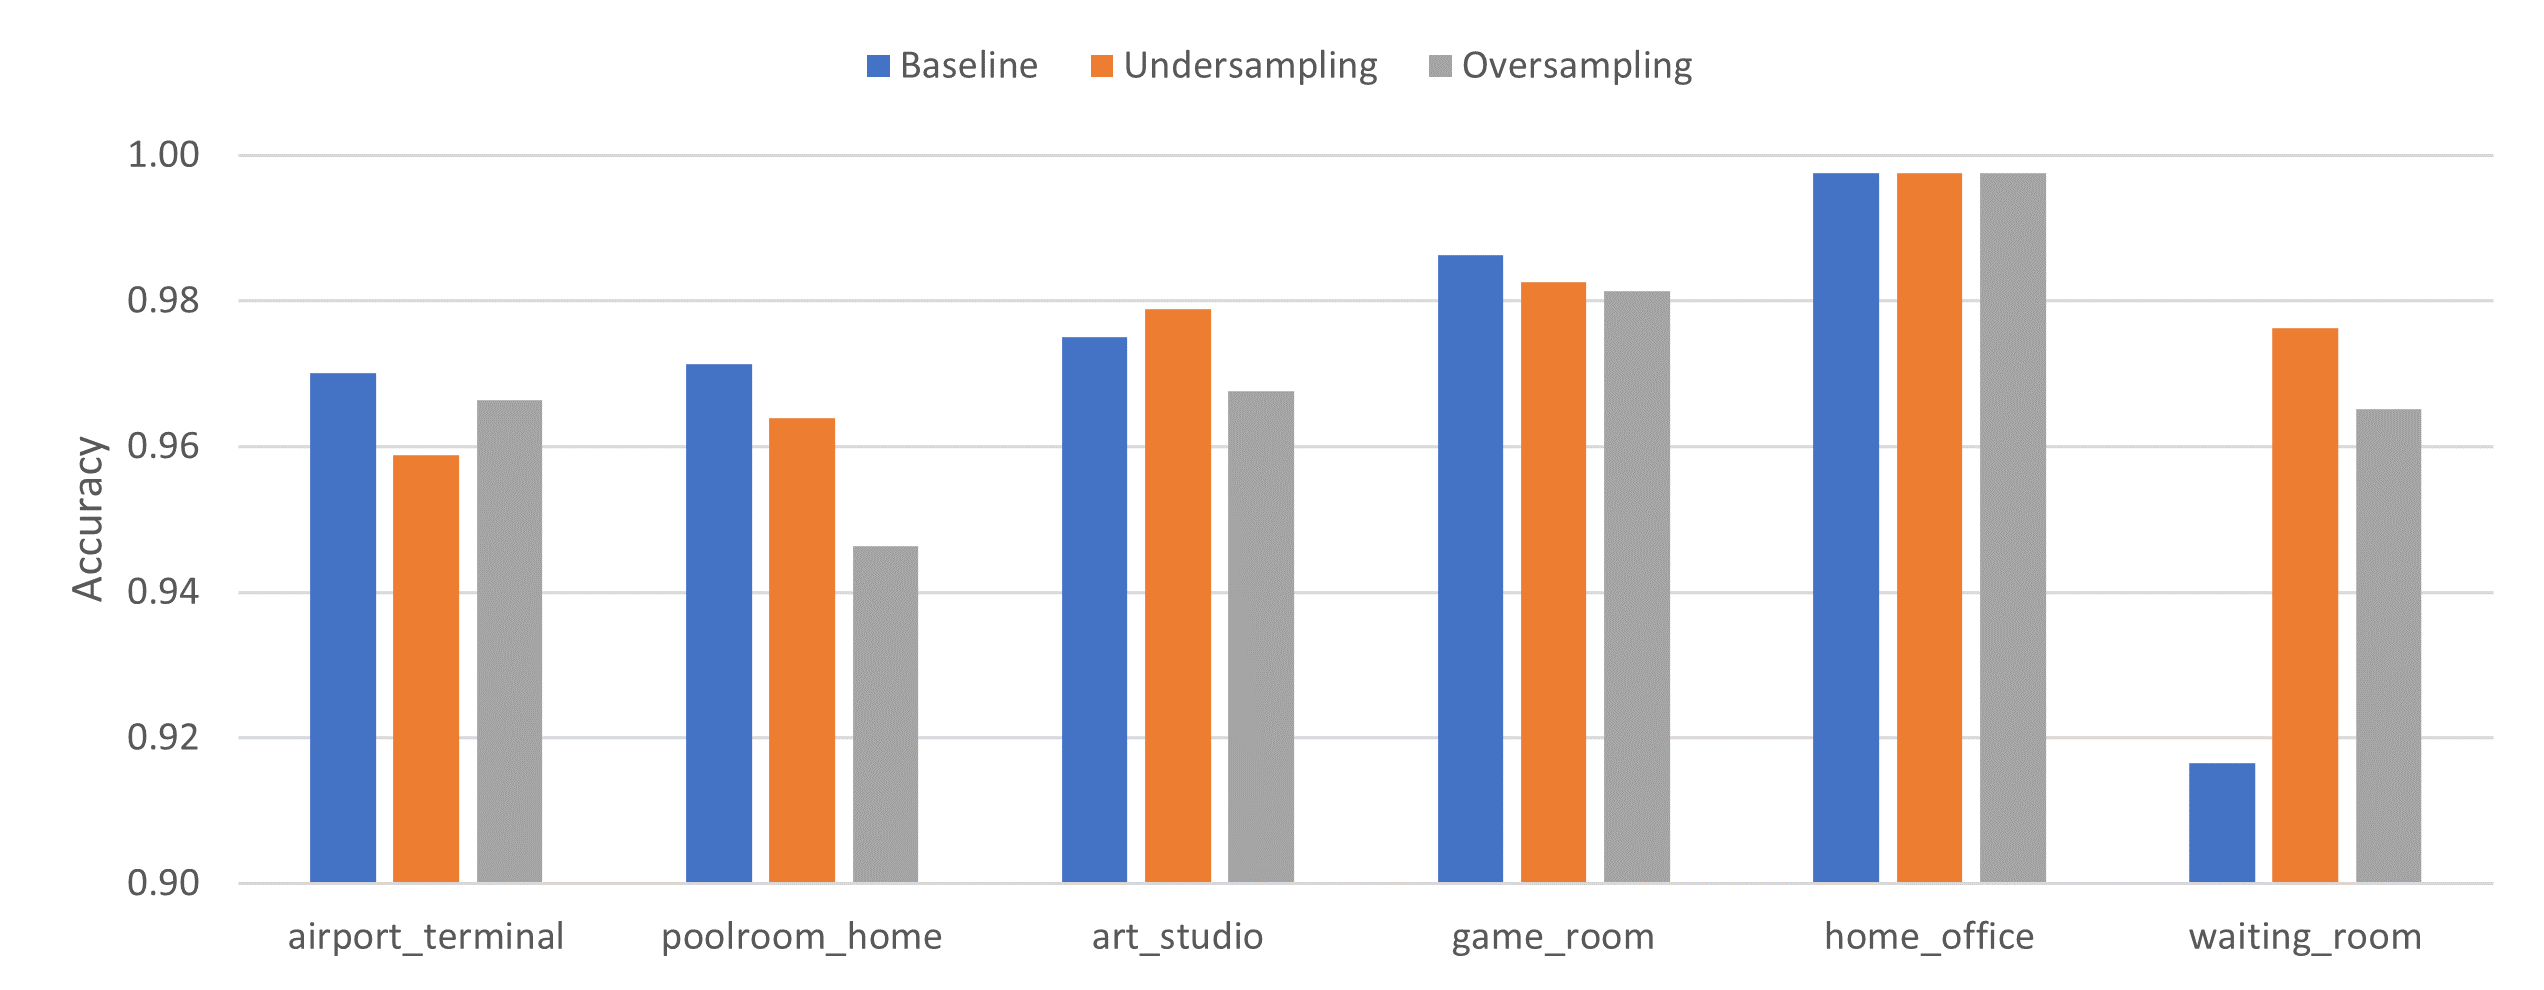}
         \caption{\textbf{Resampling accuracy on ADE20K's low-frequency classes with CLIP encoder.}}
         \label{fig:clip_ade_samp}
    \end{subfigure}

    \begin{subfigure}{0.6\linewidth}
         \centering
         \includegraphics[width=\linewidth]{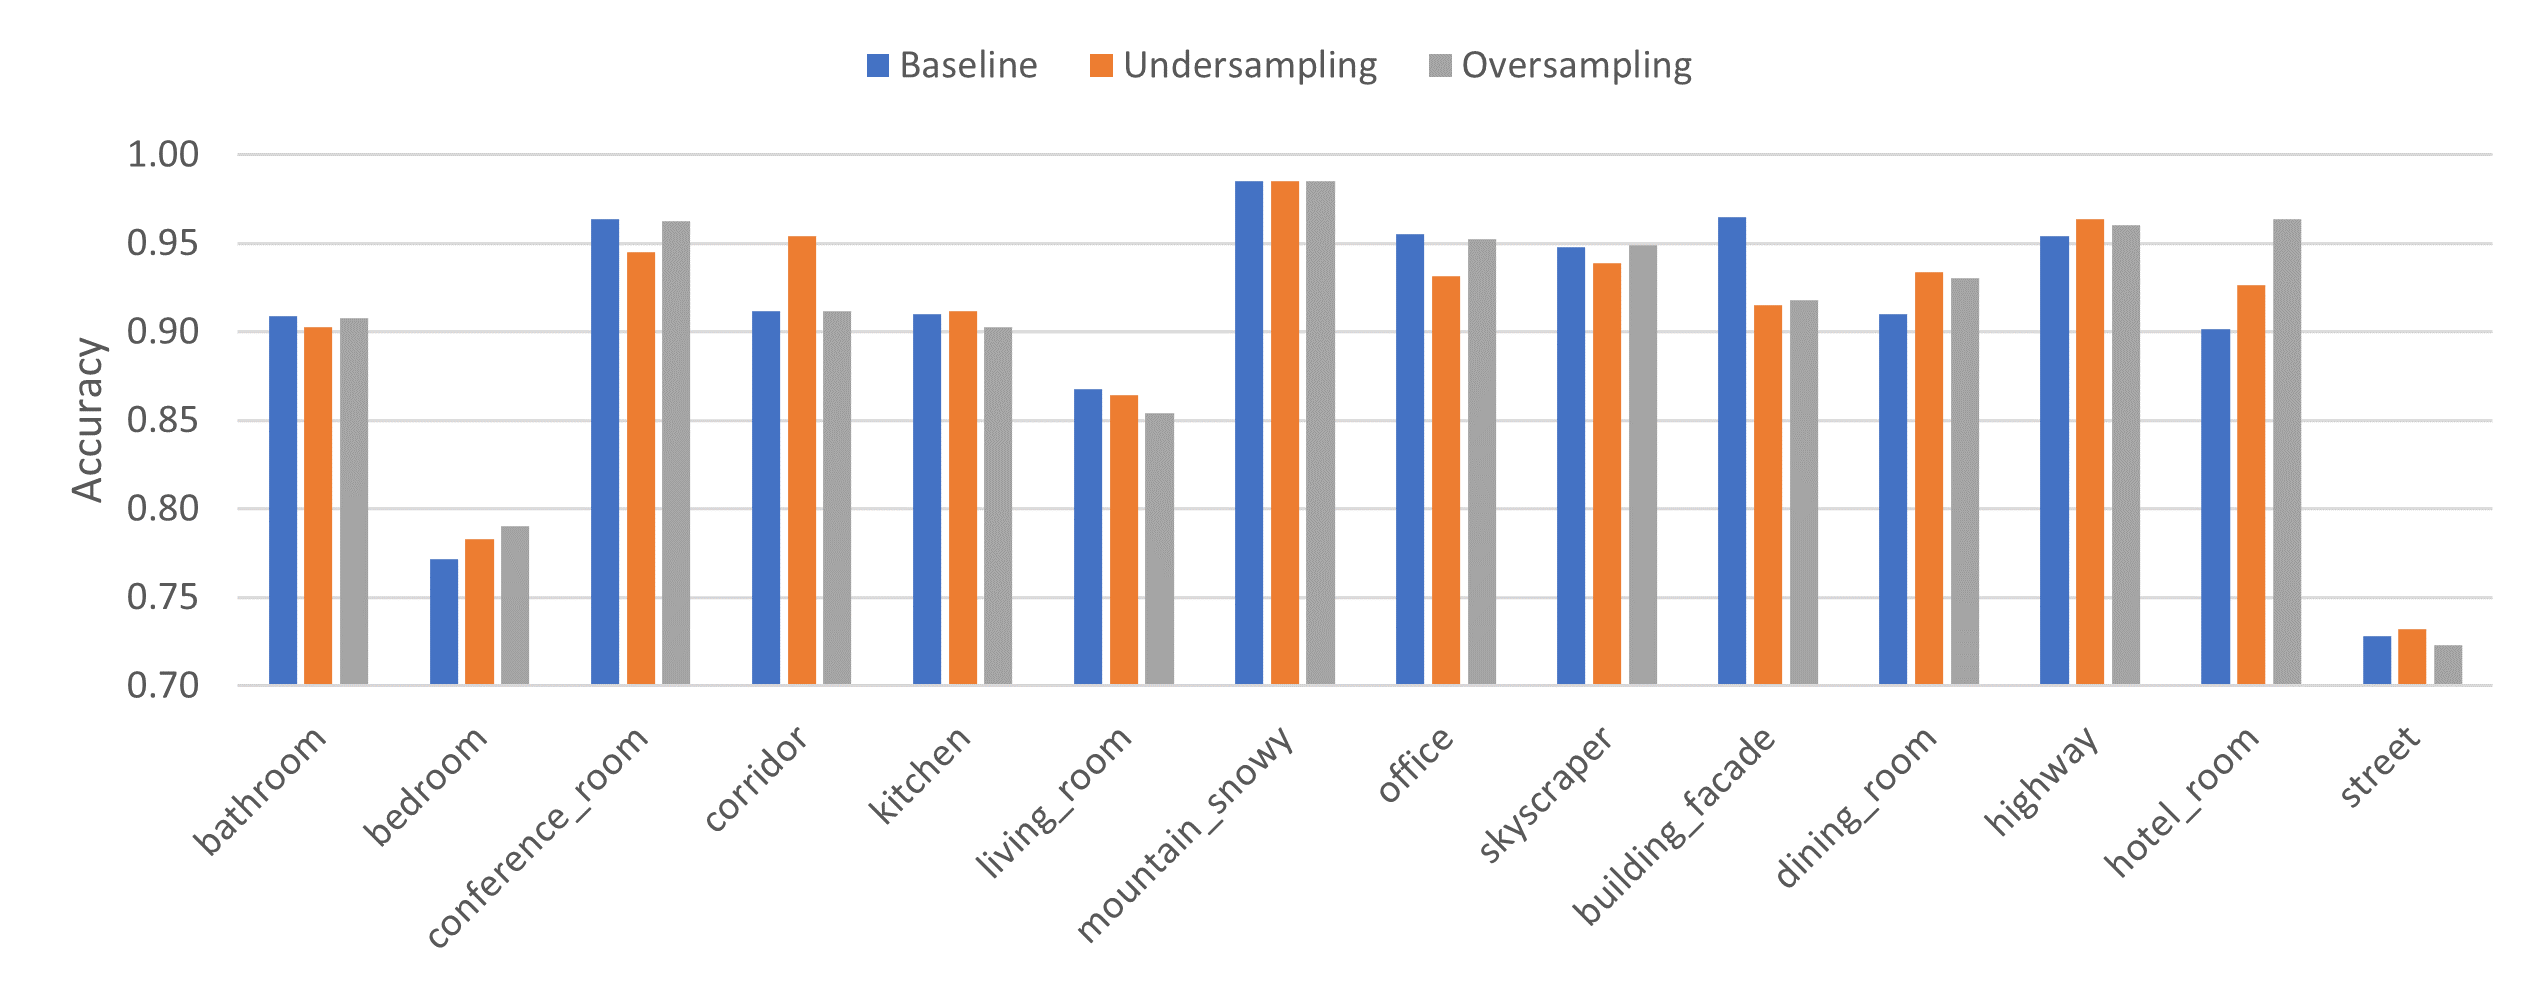}
         \caption{\textbf{Resampling accuracy on ADE20K's remaining classes with CLIP encoder.}}
         \label{fig:clip_ade_samp_nr}
    \end{subfigure}
    \caption{\textbf{Resampling accuracy on the ADE20K dataset.}}
    \label{fig:resample_results_ade}
\end{figure}

Since ADE20K involves single-label classification, the resulting distributions were exactly uniform, using $98$ for undersampling and $2,241$ for oversampling.

% \begin{figure}[h!]
% \centering
%     \begin{subfigure}{0.49\linewidth}
%         \centering
%          \includegraphics[width=\linewidth]{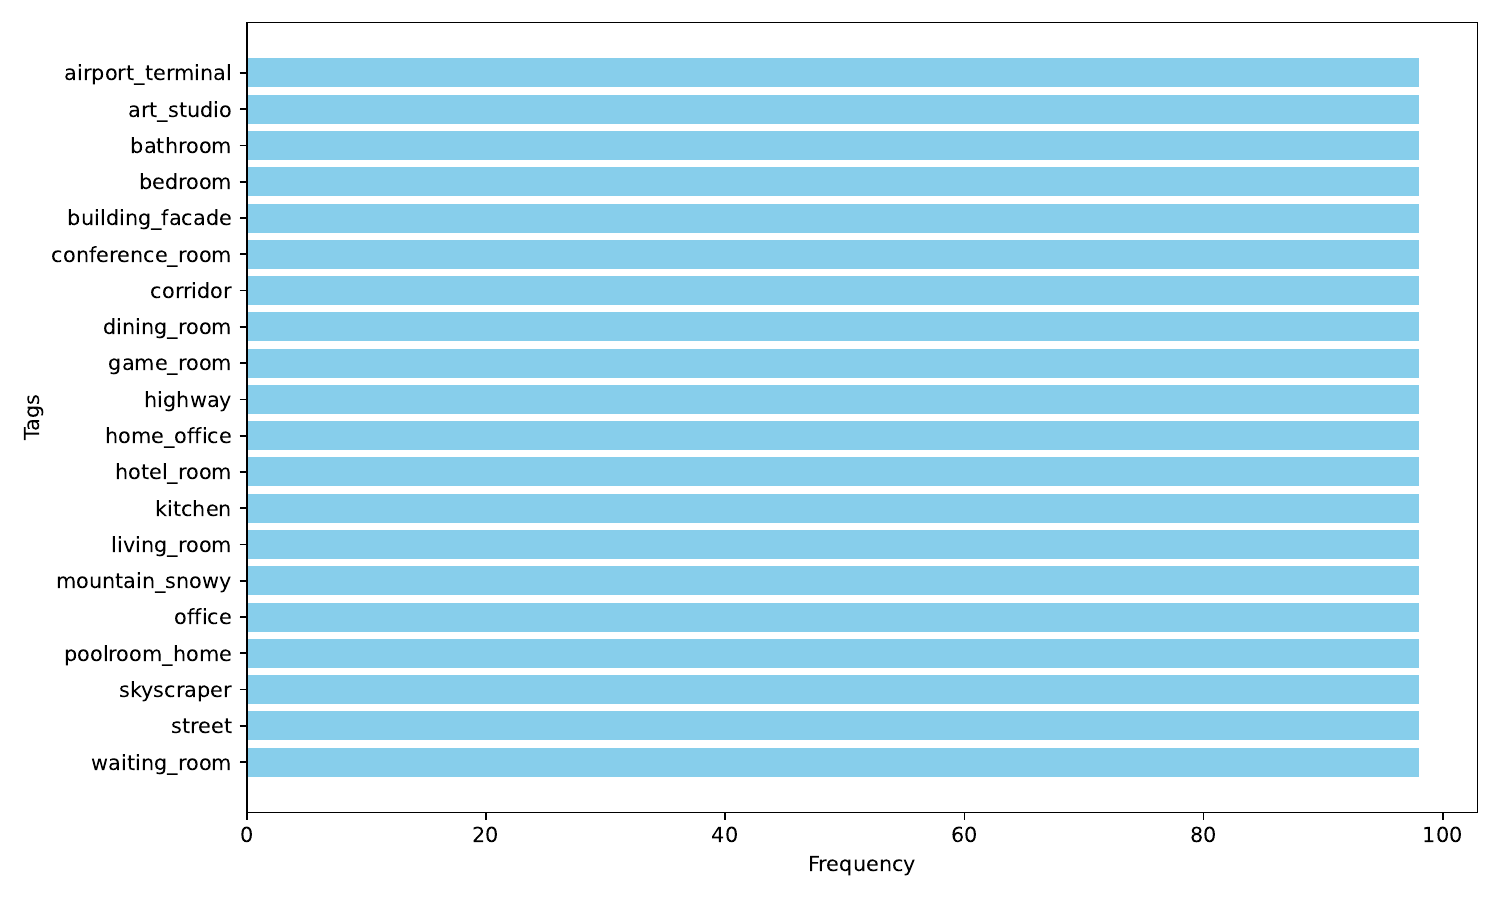}
%          \caption{\textbf{Undersampled distribution of the ADE20K dataset.}}
%          \label{fig:ade_undersamp_dist}
%     \end{subfigure}
%     \hfill
%     \begin{subfigure}{0.49\linewidth}
%         \centering
%          \includegraphics[width=\linewidth]{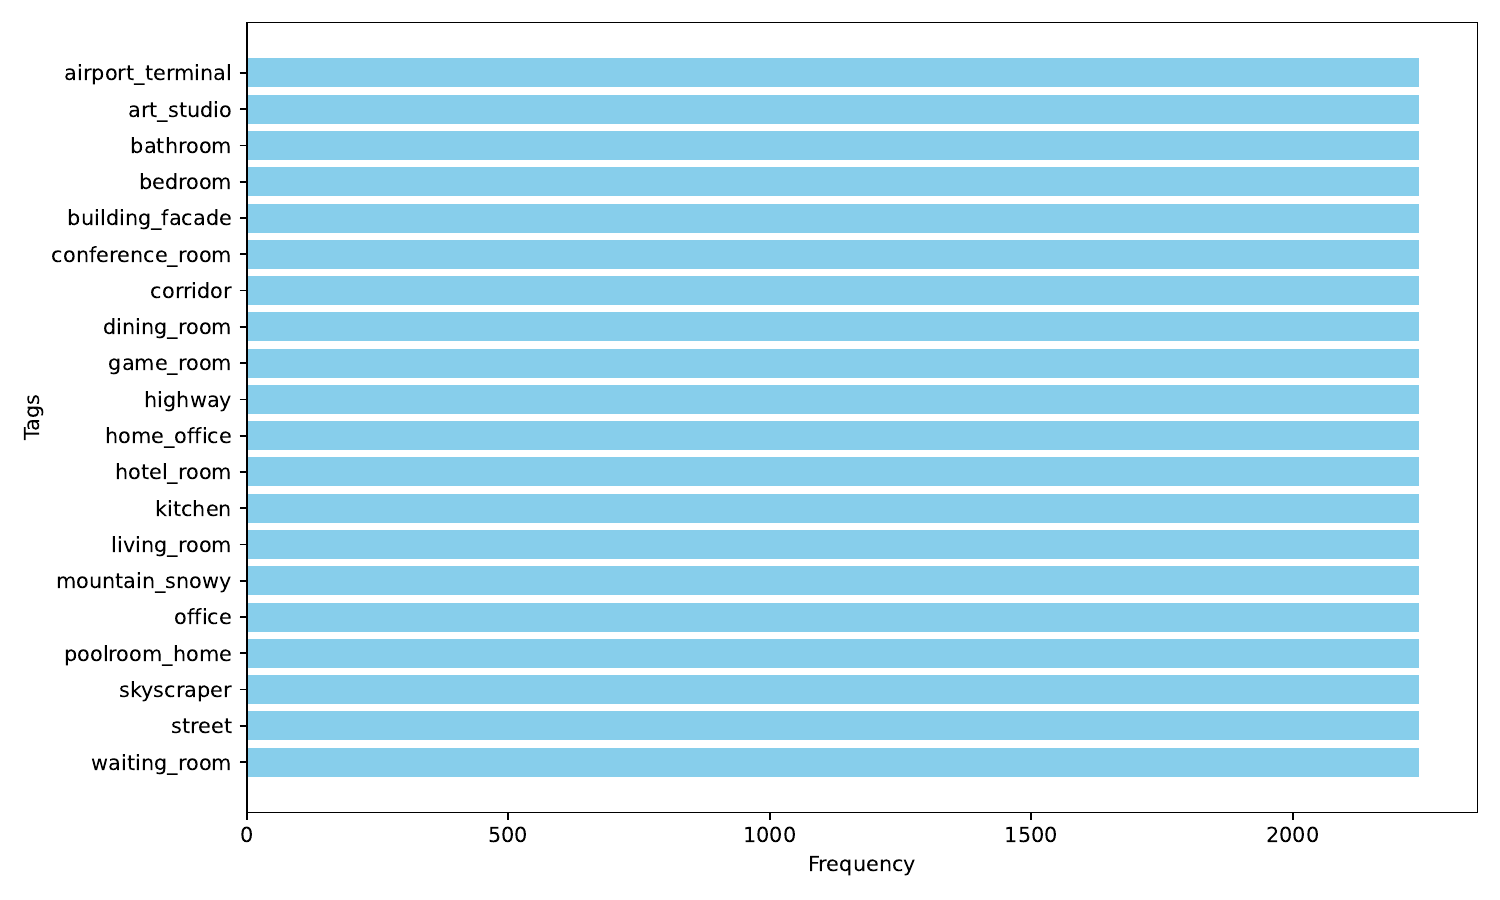}
%          \caption{\textbf{Oversampled distribution of the Planet dataset.}}
%          \label{fig:ade_oversamp_dist}
%     \end{subfigure}

%     \caption{\textbf{Resampled distributions of the ADE20K dataset.}}
%     \label{fig:ade_resample_dist}
% \end{figure}
